# Supplementary material for: On integrability of certain rank 2 sub-Riemannian structures
Source: arXiv:1507.03082 ancillary file (2016-06-17)
Supplement: Supplementary file 5 [file Worksheet_BKAVGLG-8D.pdf]

MAPLE WORKSHEET FOR THE PAPER  
 ``On integrability of certain rank 2 sub-Riemannian structures''  
 by Boris Kruglikov, Andreas Vollmer, Georgios Lukes-Gerakopoulos  
 contact e-mail: andreas.d.vollmer@gmail.com

This Maple worksheet is the implementation of the method described in the paper.  
 A previous version of the algorithm is provided in the paper preprint arXiv:1507.03082 and in the thesis ``First integrals in stationary and axially symmetric space-times and sub-Riemannian structures'' by the second author (AV). The worksheet is based on a Maple worksheet by V. Matveev and the first author (BK), which can be found as supplement material to the paper ``Nonexistence of the 6th degree integral for Zipoy-Voorhees metric'', Phys. Rev. D 85(2012).

**Purpose:**

Given a sub-Riemannian metric on a rank-2 distribution on a Carnot group, the worksheet determines an upper bound to the number of first integrals that are homogeneous polynomials in the momenta with smooth coefficient functions. By comparing this bound to the number of trivial integrals, non-existence of non-trivial integrals is confirmed. Certain involutivity assumptions are made. See the paper for details.

```
> restart;
> with(LinearAlgebra):
> startclock := time();

                                startclock := 1.075401578 106 (1)
```

**Parameter input:**

The following data have to be provided:

- (1) dimension **N** of the Carnot group
- (2) degree **d** of the integral
- (3) number **M** of prolongations (we achieve our results after d+1 prolongations)
- (4) choice of the rank computation algorithm by setting **algorithmchoice**.  
 The choices are "bareiss" (Bareiss algorithm), "gauss" (Gauß algorithm) oder "modular" (computations modulo *prim*).
- (5) a prime number **prim**. It is only used in case of modular rank computation, and in this case the final steps are performed modulo *prim*.
- (6) the Hamiltonian **H** representing the sub-Riemannian metric. Set the corresponding variable below.

```
> N:=8;
   d:=5;
   M:=d+1;
   algorithmchoice:="gauss";
   prim:=17;

                                N := 8
                                d := 5
                                M := 6
                                algorithmchoice := "gauss"
                                prim := 17 (2)
```

The following information are system variables that should not be changed.

x denotes the position coordinates, while p denotes the momentum coordinates.

```
> x:=array(1..N):
> p:=array(1..N):
```

In the following, the left-invariant Hamiltonians are defined. They are given by  $H=1/2*(X1^2+X2^2)$ .

Do not change these entries, but rather change the selection of H below.

6D parabolic metric

```
> if N=6 then
    H6Dp:= 1/2*((p[1]-(1/2)*x[2]*p[3]-x[1]*x[2]*p[4]-(1/2)*x[1]^2*
x[2]*p[6])^2+(p[2]+(1/2)*x[1]*p[3]+x[1]*x[2]*p[5])^2):
fi:
```

6D hyperbolic metric

```
> if N=6 then
    H6Dh:= 1/2*((p[1]-(1/2)*x[2]*p[3]-x[1]*x[2]*p[4]-(1/4)*x[1]*x
[2]^2*p[6])^2+(p[2]+(1/2)*x[1]*p[3]+x[1]*x[2]*p[5]+(1/4)*x[1]^2*x
[2]*p[6])^2):
fi:
```

7D metric

```
> if N=7 then
    H7D := 1/2*((p[1]-(1/2)*x[2]*p[3]-x[1]*x[2]*p[4]-(1/2)*x[1]^2*
x[2]*p[6]-(1/4)*x[1]*x[2]^2*p[7])^2+(p[2]+(1/2)*x[1]*p[3]+x[1]*x
[2]*p[5]-(1/2)*x[1]*x[2]^2*p[6]+(1/4)*x[1]^2*x[2]*p[7])^2):
fi:
```

8D metric

```
> if N=8 then
    H8D:= 1/2*((p[1]-(1/2)*x[2]*p[3]-((x[1]^2+x[2]^2)*(1/2))*p[5]-
(1/4)*x[1]*x[2]^2*p[7]-(1/6)*x[2]^3*p[8])^2+(p[2]+(1/2)*x[1]*p[3]
+((x[1]^2+x[2]^2)*(1/2))*p[4]+(1/6)*x[1]^3*p[6]+(1/4)*x[1]^2*x[2]
*p[7])^2):
fi:
```

### Definition of sub-Riemannian structure (Hamiltonian):

Enter/Choose the Hamiltonian for the case to consider.

```
> H:=H8D;
```

$$H := \frac{1}{2} \left( p_1 - \frac{1}{2} x_2 p_3 - \frac{1}{2} (x_1^2 + x_2^2) p_5 - \frac{1}{4} x_1 x_2^2 p_7 - \frac{1}{6} x_2^3 p_8 \right)^2 + \frac{1}{2} \left( p_2 + \frac{1}{2} x_1 p_3 + \frac{1}{2} (x_1^2 + x_2^2) p_4 + \frac{1}{6} x_1^3 p_6 + \frac{1}{4} x_1^2 x_2 p_7 \right)^2 \quad (3)$$

## Definition of routines

In order to make the code universal and readable, we define a number of routines.

### generateCases

Purpose: generate a set of *loops* integers that add up to a given integer *limit*. Needed to obtain all possible combinations of momenta that appear in an integral.

Takes two integers, *limit* (the fixed sum of the integers) and *loops* (the number of integers to be generated in each example).

Returns a list of possible sets of *loops* many integers that add up to *limit*.

```
> generateCases:=proc(limit::integer,loops::integer)::list;
    local store::list, mem::list,el,l,t;
    store:=[seq([l],l=0..limit)];
    for l from 1 to loops-2 do:
        mem:=[]:
        for el in store do:
            mem:=[op(mem),seq([op(el),l],l=0..(limit-add(el[t],t=1..nops
(el))))];
        od:
        store:=mem:
    od:
    mem:=map(Q->[op(Q),limit-add(Q[1],l=1..nops(Q))], store);
```

```

return mem:
end proc:

```

### **lterm**

Purpose: find the leading term of a polynomial

Takes two arguments, *polynomeqn* (a polynomial) and *vars* (a list of variables)

Returns the leading term (coefficient multiplied with monomial) of *polynomeqn* w.r.t. the variables *vars*.

```

> lterm:=proc(polynomeqn,vars):
    return lcoeff(polynomeqn,vars,'lm')*lm:
end proc;
lterm := proc(polynomeqn,vars) return lcoeff(polynomeqn,vars,'lm')*lm end proc (4)

```

### **tterm**

same as lterm, but computes the trailing term instead of the leading term.

```

> tterm:=proc(polynomeqn,vars):
    return tcoeff(polynomeqn,vars,'lm')*lm:
end proc;
tterm := proc(polynomeqn,vars) return tcoeff(polynomeqn,vars,'lm')*lm end proc (5)

```

### **hasMonomial**

Purpose: determine whether a list of equations contains an equation monomial in a set of variables

Takes *eqns* (a list of polynomial expressions) and *vars* (a list of variables)

Returns a boolean value: true if there is a monomial equation in the system w.r.t. *vars*; false if not.

```

> hasMonomial:=proc(eqns::list,vars)::boolean;
    local i;
    for i from 1 to nops(eqns) do
        if eqns[i]=lterm(eqns[i],vars) and eqns[i]<>0 then
            return true;
        fi:
    od:
    return false:
end proc:

```

### **hasBimonomial**

same as hasMonomial, but looks for bi-monomial equations.

```

> hasBimonomial:=proc(eqns::list,vars)::boolean;
    local i;
    for i from 1 to nops(eqns) do
        if eqns[i]=lterm(eqns[i],vars)+tterm(eqns[i],vars) and eqns
[i]<>0 then
            return true;
        end if:
    od:
    return false:
end proc:

```

### **solveMonomialEqns**

Purpose: partially solve a system of equations using the monomial equations

Takes two arguments: *inputeqns* (a list of equations) and *vars* (a list of variables)

Returns a list of equations (this is the partially solved system); the obtained solutions are stored in the global set *monomialeqns*.

```

> solveMonomialEqns:=proc(inputeqns::list,vars)::list;
    global monomialeqns;
    local i, flag, eqns;
    flag:=true:
    eqns:=inputeqns:
    while flag=true do:
        for i from 1 to nops(eqns) do:

```

```

    if eqns[i]=lterm(eqns[i],vars) and eqns[i]<>0 then:
      monomialeqns:={op(monomialeqns),eqns[i]/lcoeff(eqns[i],
vars)}}:
      eqns:=subs(eqns[i]/lcoeff(eqns[i],vars)=0, eqns):
      fi:
    od:
    #print("done: monomial cycle"):
    flag:=false:
    for i from 1 to nops(req) do:
      if eqns[i]=lterm(eqns[i],vars) and eqns[i]<>0 then
        flag:=true:
        break:
      end if:
    od:
  od:
  return eqns:
end proc:

```

### **solveBimonomialEqns**

As solveMonomialEqns, but for bimonomial equations.

```

> solveBimonomialEqns:=proc(inputeqns::list,vars)::list;
  global binomialeqns;
  local i, flag, eqns, leadmon;
  flag:=true:
  eqns:=inputeqns:
  while flag=true do:
    for i from 1 to nops(eqns) do:
      if eqns[i]=lterm(eqns[i],vars)+tterm(eqns[i],vars) and
eqns[i]<>0 then:
        leadmon:=[lcoeff(eqns[i],vars,'m'),m]:
        binomialeqns:={op(binomialeqns),leadmon[2]}:
        eqns:=subs(leadmon[2]=-tterm(eqns[i],vars)/leadmon[1],
eqns):
      end if:
    od:
    #print("done: binomial cycle"):
    flag:=false:
    for i from 1 to nops(eqns) do:
      if eqns[i]=lterm(eqns[i],vars)+tterm(eqns[i],vars) and
eqns[i]<>0 then:
        flag:=true:
        break:
      end if:
    od:
  od:
  return eqns:
end proc:

```

### **reduceList**

Purpose: reduce a list of given equations (polynomial expressions) by removing duplicates

Takes a list of polynomial expressions

Returns a list of polynomial expressions

```

> reduceList:=proc(eqns::list)::list;
  {op(eqns)}:
  return [op(%)]:
end proc:

```

## Computation of the associated system

In this section, we define the integral and compute the system of PDEs encoding the requirement that a given polynomial in the momenta is an integral.

The integral is a homogeneous polynomial of the degree  $d$ , which has been specified above.

$F_{\text{trivials}}$  is the set of coefficients of the integral that can be set to zero (in a point) by subtraction of (constant multiples) of trivial/standard integrals

```
> a:=array(seq(0..d,i=1..N-1)):
> coefficient:={}:
  for i from 0 to d do:
    for j from 0 to i do:
      for el_k in generateCases(d-i,N-2) do:
        coefficient:={op(coefficient), a[i,j,op(1..N-3,el_k)]=a[i,j,
op(1..N-3,el_k)](x[1],x[2])}:
      od:
    od:od:
  alias(op(coefficient)):
> F:=0:
  for i from 0 to d do:
    for j from 0 to i do:
      for el_k in generateCases(d-i,N-2) do:
        F:=F+a[i,j,op(1..N-3,el_k)](x[1],x[2])*p[1]^j*p[2]^(i-j)*
product(p[1]^el_k[1-2],l=3..N);
      od:
    od:od:
> F_trivials:={}:
  for i from 0 to d by 2 do:
    for el_k in generateCases(d-i,N-2) do:
      F_trivials:= F_trivials union {a[i,0,op(1..N-3,el_k)](x[1], x
[2])}:
    od:od:
```

Now compute the Poisson bracket between the Hamiltonian and the integral.

Derive from it the corresponding equational system by taking derivatives w.r.t. momenta.

$Eq$  is the set of equations on the unknown functions (which are the components of  $F$ ).

```
> Pois:= 0:
  for i to N do:
    Pois:=Pois+diff(H,x[i])*diff(F,p[i])-diff(F,x[i])*diff(H,p[i]):
  od:
  Pois:= simplify(Pois):
> Eq:={}:
  for i from 0 to (d+1) do
    for j from 0 to (d+1-i) do
      for el_k in generateCases(d+1-i-j,N-2) do
        tmp:= diff(Pois, p[1]$i,p[2]$j,seq(p[w+2]$el_k[w],w=1..N-2)):
        if tmp<>0 then Eq:= {op(Eq),tmp } end if:
      od:od:od:
```

Prolongation step.

The first  $M$  prolongations are computed. The result is the set  $DEq$  of differential equations.

$DEq$  is obtained by taking  $0,1,\dots,M$  derivatives of  $Eq$  w.r.t.  $x[1]$  and  $x[2]$ .

```
> DEq:= Eq:
  for m to M do:
    for i from 0 to m do:
      DEq:= {op(DEq), op(diff(Eq, x[1]$i, x[2]$(m-i)))}:
    od:
  od:
```

**od:od:**

The set **var** contains all coefficients of F which are unknowns of the differential system DEq. **dvar** is the corresponding set of all unknowns including derivatives of entries of **var**. **dvar** is the set of unknown functions in our system of linear equations.

The variable **subvar** is necessary to implement the unknowns as variables, since var contains the **a[...]** which are functions.

The arguments in **subvar** are

- (1) Number of derivatives w.r.t.  $x[1]$
- (2) Ordinal of the variable/unknown function (as obtained from **var**)
- (3) Total number of derivatives (--> connected with number of prolongations performed)

```
> var:={}:
  for i from 0 to d do
    for j from 0 to i do
      for el_k in generateCases(d-i,N-2) do
        var := {op(var), a[i,j,seq(el_k[1-2],l=3..N-1)](x[1], x[2])
      }
    od:od:od:
  > sub:= {}:
  subvar:= array(0..M+1,0..nops(var),0..M+1):
  dvar:={}:
  for n from 0 to M do:
    m:= M+1-n:
    for i from 0 to m do
      for j to nops(var) do
        sub:= {op(sub), diff(var[j], x[1]$i, x[2]$(m-i))=subvar[i,j,
m] }:
        dvar:= {op(dvar), subvar[i,j,m]}:
      od:
    od:
  DEq:= subs(sub, DEq):
od:
```

Now, we replace the derivatives of the unknown functions (and the functions themselves) by variables from **subvar** (which are not functions).

The unknown functions are **var[1].var[...]**, and they and their derivatives are labelled by subvar:

**subvar[i,j,m]** is the  $(x[1]^i, x[2]^{(m-i)})$ -derivative of **var[j]**.

The corresponding list is dvar.

Most of this has already been done in the previous step. Now we add "zeroth derivatives", i.e. we add the unknown functions in var themselves to **dvar** and **subvar**, and we replace them in **DEq**.

Coefficients in **DEq** are functions.

```
> for j to nops(var) do:
  sub:= {op(sub), var[j]= subvar[0,j,0]}:
  dvar:= {op(dvar), subvar[0,j,0]}:
od:
DEq:= subs(sub, DEq):
```

We count the number of equations as well as the number of unknowns (entries of **DEq** and **dvar** respectively)

```
> nops(DEq); nops(dvar);
```

48048

28512

(6)

We convert the coefficients that can be set to zero to the algebraic convention

```
> dvar_trivials:=subs(sub,F_trivials):
  sub_trivials:=map(Q->Q=0, dvar_trivials):
```

Now we specify a certain point on the sub-Riemannian piece (i.e. we specify  $x_1$  and  $x_2$  only):

- (1) we substitute  $x[1]$  and  $x[2]$  by numerical values  
--> we call the resulting system of equations **deq**
- (2) **deq** is a system of linear equations in the unknowns (listed in **dvar**)
- (3) coefficients in **deq** are numbers (in **DEq** it were expressions)

```
> deq:= subs(x[1]= 0, x[2]= 0, DEq):
> deq:= subs(sub_trivials, deq):
```

## Reduction of the associated system

To reduce the number of equations to deal with, 'normalize' the coefficients and 'integerize' them to make computations faster (coefficients in ZZ instead of QQ).

In case of the choice *algorithmchoice="modular"*, the equations are taken modulo *prim*.

```
> tmpeq:={}:
  if algorithmchoice="modular" then
    for i from 1 to nops(deq) do
      if deq[i]<>0 then tmpeq:={op(tmpeq),numer(expand(deq[i]
/lcoeff(deq[i],dvar))) mod prim} fi:
    od:
  else
    for i from 1 to nops(deq) do
      if deq[i]<>0 then tmpeq:={op(tmpeq),numer(expand(deq[i]
/lcoeff(deq[i],dvar)))} fi:
    od:
  fi:
deq:=tmpeq:
nops(deq);
```

45249

(7)

Remove all variables that do not appear in any of the equations (in the corresponding matrix, these are columns with vanishing entries).

- (1) The list **superfluent** contains all does "redundant" variables
- (2) All the other variables are stored in the **necessary** list. Later we call this list **Nvar**.

```
> superfluent:=[]:
  necessary:=[]:
  for i from 1 to nops(dvar) do:
    flag:=convert({seq(coeff(deq[j],dvar[i]),j=1..nops(deq))}={0},
truefalse):
    if flag=true then
      superfluent:=[op(superfluent),dvar[i]]:
    else
      necessary:=[op(necessary),dvar[i]]:
    end if:
  od:
nops(superfluent);
nops(necessary);
```

314

28198

(8)

```
> avar:=dvar:
dvar:=necessary:
```

Final simplification/reduction step: solve the (trivial) equations that are monomial and binomial. Their variables have later to be added to the number of unknowns, and the number of respective equations has to be added to the rank. Thus, no corrections are necessary since both effects/corrections cancel out



```

    if deq[i]<>0 then
      req:={op(req),numer(expand(deq[i]/lcoeff(deq[i],dvar))) mod
prim}:
    end if:
  od:
else
  for i from 1 to nops(deq) do:
    if deq[i]<>0 then
      req:={op(req),numer(expand(deq[i]/lcoeff(deq[i],dvar)))}:
    end if:
  od:
fi:
deq:=req:
nops(deq);

```

4439 (12)

Finally, remove trivial equations (if any) and compile the set of remaining variables (removing the unknowns addressed for by the reduction procedure).

The number of remaining equations and variables gives the size of the matrix for which we have to compute the rank.

```

> deq:={op(deq)} minus {0}:
> dvar:={op(dvar)} minus monomialeqns minus binomialeqns:
> nops(deq);
nops(dvar);

```

4439  
3514 (13)

We determine the matrix of coefficients of the equations (listed in **deq**) w.r.t. the unknowns (entries in **dvar**).

**Mat** is the matrix of the system of equations established above. Its entries are numbers.

```

> Mat:= Matrix(nops(deq), nops(dvar)):
  for i to nops(deq) do
    for j to nops(dvar) do
      Mat[i,j]:= coeff(deq[i],dvar[j]):
    od:od:
> rows:=RowDimension(Mat);
cols:=ColumnDimension(Mat);
rows,cols;

```

rows := 4439  
cols := 3514  
4439, 3514 (14)

The result of this computation yields: **rk**: The rank of **Mat**

We implement three possible rank computation schemes: the usual Gauss algorithm, the Bareiss algorithm, and a modular Gauss algorithm.

In the modular case, one needs to specify the prime modulus **prim** in the beginning.

**Caveat:** Two problems may occur and force one to rerun the code: (i) If **prim** is too small, an error alert will appear if it is impossible to perform modular inversion. In this case, choose a larger prime and rerun the code. (ii) If the resulting number of additional integrals is nonzero, the reason might be that the rank of **Mat** has dropped because we are using modular arithmetic, not because the initial matrix has lower rank. So, this needs not be a hint to the existing of additional integrals. Choose another prime, or another algorithm to check it.

```

> if algorithmchoice="bareiss" then
  Z[0],Z[1],Z[+],Z[-],Z[*],Z[=]:=0,1,+,-,* , = :

```

```

Z[Divide] := proc(a,b,q) evalb( irem(args) = 0 ) end proc:
Mat2:=LinearAlgebra:-Generic:-BareissAlgorithm[Z](Mat):
rk:=numelems(RowSpace(Mat2)):
print("Bareiss");
elif algorithmchoice="modular" then
  #Rowreduce(p, A, rows, cols, rcol, det, pdet, rank, sig,
incrow, redflag)
  if cols=0 or rows=0 then
    rk:=0:
  else
    AMat:=LinearAlgebra:-Modular:-Copy(prim,Mat):
    LinearAlgebra:-Modular:-RowReduce(prim,AMat,rows,cols,cols,0,
0,'rk',0,0,false):
    fi:
    print("Modular");
  else
    rk:=Rank(Mat):
    print("Gauss");
  fi:

```

"Gauss" (15)

**Delta** is the dimension of the space of solutions for the original problem.  
Note that contributions from 'monomialeqns' cancel out, so only 'superfluent' has to be taken into account when computing Delta.

```

> print("Delta=",nops(superfluent)+nops(dvar)-rk);

```

"Delta=", 314 (16)

We track the time and compute the time period needed to perform the computation.

```

> stopclock := time();

```

*stopclock := 1.119062625 10<sup>6</sup>* (17)

## Results

```

> ['M'=M, 'd'=d];

```

[M=6, d=5] (18)

### Computation time

```

> time_used := stopclock-startclock:
> hrs:=floor((1/3600)*time_used);
mins:=floor((time_used-3600*hrs)*(1/60));
secs:=time_used-3600*hrs-60*mins;

```

*hrs := 12*  
*mins := 7*  
*secs := 41.047* (19)

### initial dimensions of the system

```

> print('equations', nops(DEq));
print('unknowns', nops(avar));

```

*equations, 48048*  
*unknowns, 28512* (20)

### dimensions after reduction & rank

```

> print('equations', nops(deq));
print('unknowns', nops(dvar));

```

*equations, 4439*  
*unknowns, 3514* (21)

```
> print('rank', rk);
```

*rank*, 3514 (22)

```
> print('superfluent', nops(superfluent));
print('necessary', nops(necessary));
```

*superfluent*, 314  
*necessary*, 28198 (23)

```

                                final result
> print('Delta', nops(superfluent)+nops(dvar)-rk);
unassign('i'): sum( binomial(N+d-2*i-3, N-3), i=0..floor(d/2) ):
print('Delta', '(trivial)', % );
print('nontrivials', nops(superfluent)+nops(dvar)-rk-%);
```

$\Delta$ , 314  
 $\Delta$ , *trivial*, 314  
*nontrivials*, 0 (24)

If *nontrivials* is 0, non-existence of additional integrals is proven. In case *nontrivials*  $\neq$  0, try for different number of prolongation steps, another choice of the point of reference or another prime *prim* (in case of modular computation).
